# Supplementary material for: Indicator patterns of forced change learned by an artificial neural network
Source: arXiv:2005.12322 ancillary file (2020-05-25)
Supplement: Supplementary file 1 [file Barnes_Toms_etal_2020_JAMES_SupportingInformation.pdf]

# SUPPLEMENTARY FIGURES
# Indicator patterns of forced change learned by an artificial neural network

Elizabeth A. Barnes[1], Benjamin Toms[1], James W. Hurrell[1], Imme Ebert-Uphoff[2,3], Chuck Anderson[4,5], and David Anderson[5]

[1]Department of Atmospheric Science, Colorado State University, Fort Collins, CO
[2]Cooperative Institute for Research in the Atmosphere, Colorado State University, Fort Collins, CO
[3]Department of Electrical and Computer Engineering, Colorado State University, Fort Collins, CO
[4]Department of Computer Science, Colorado State University, Fort Collins, CO
[5]Pattern Exploration LLC, Fort Collins, CO

Corresponding author: Elizabeth A. Barnes (eabarnes@rams.colostate.edu)

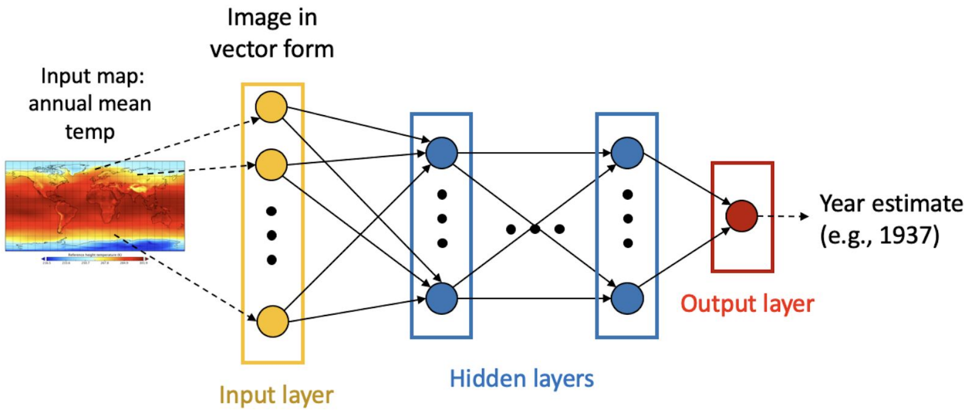


**Supp. Figure 1:** Schematic of NN architecture used in Barnes et al. (2019). The output is a single scalar, indicating the year estimated for the input map. The NN task is to estimate a continuous number, which is called a *regression* task.

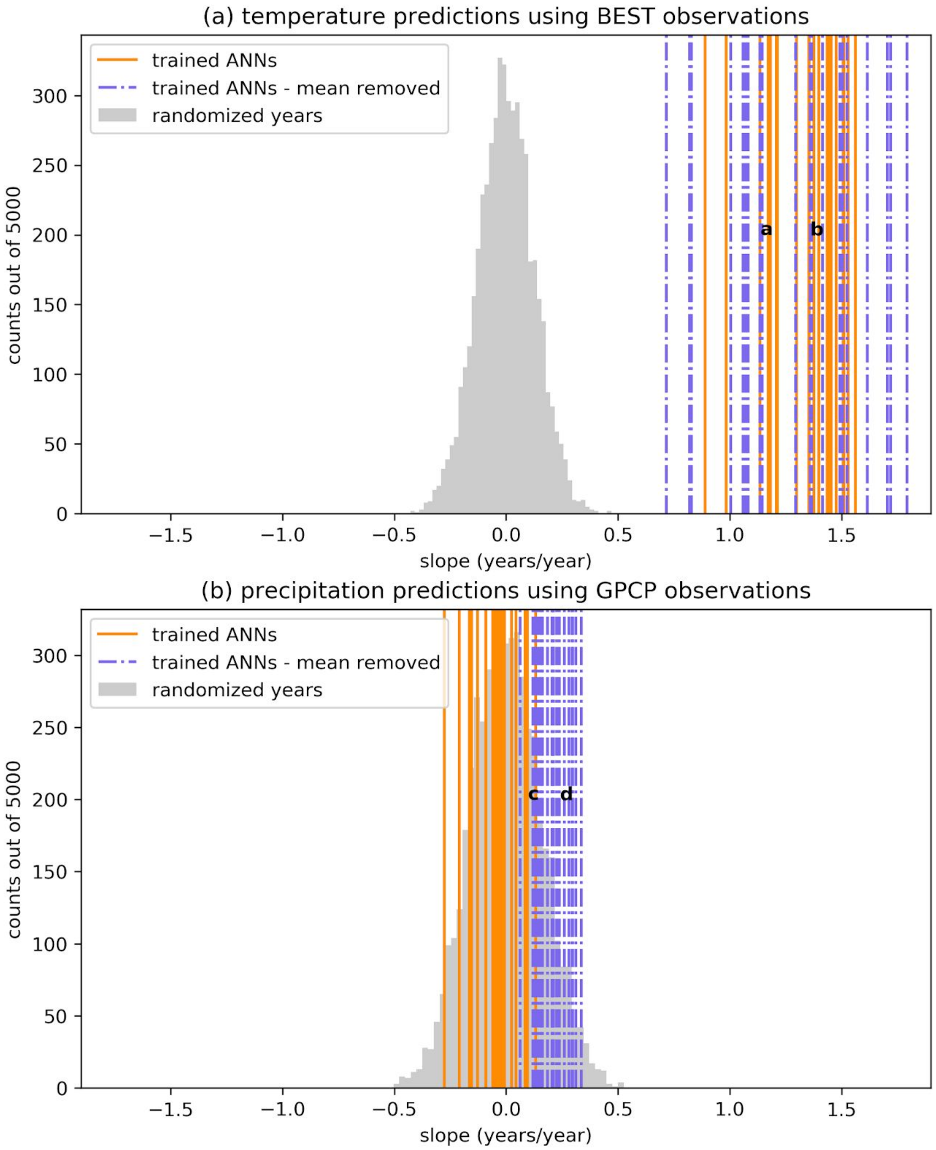


**Supp. Figure 2:** Slopes of the best-fit line between the actual years and the ANN-predicted years based on observed maps of (a) temperature and (b) precipitation. Different lines denote different iterations of training the ANN. (gray shading) Histogram of possible slopes between two time series with shuffled years (i.e. the range of correlations obtained when no relationship is present). Bold letters denote the iterations that are associated with the four panels of Fig. 3.

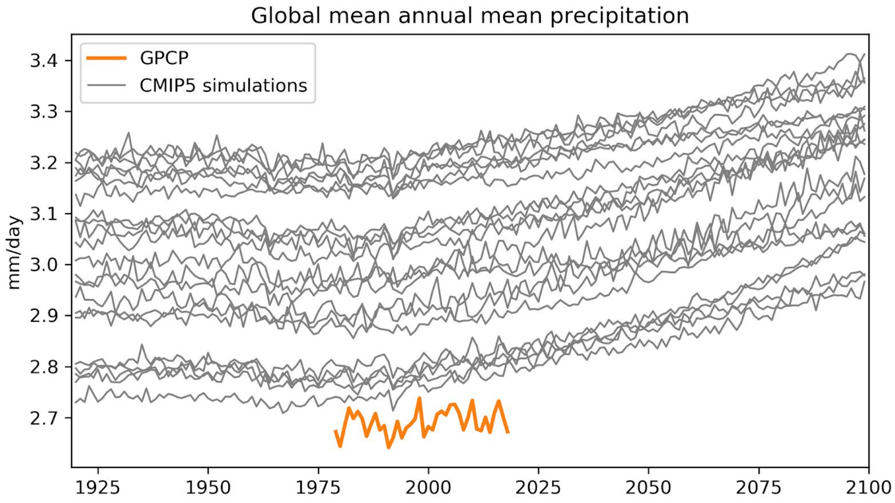


**Supp. Figure 3:** Global-mean, annual-mean precipitation as a function of year for each of the CMIP5 simulations and GPCP observations.

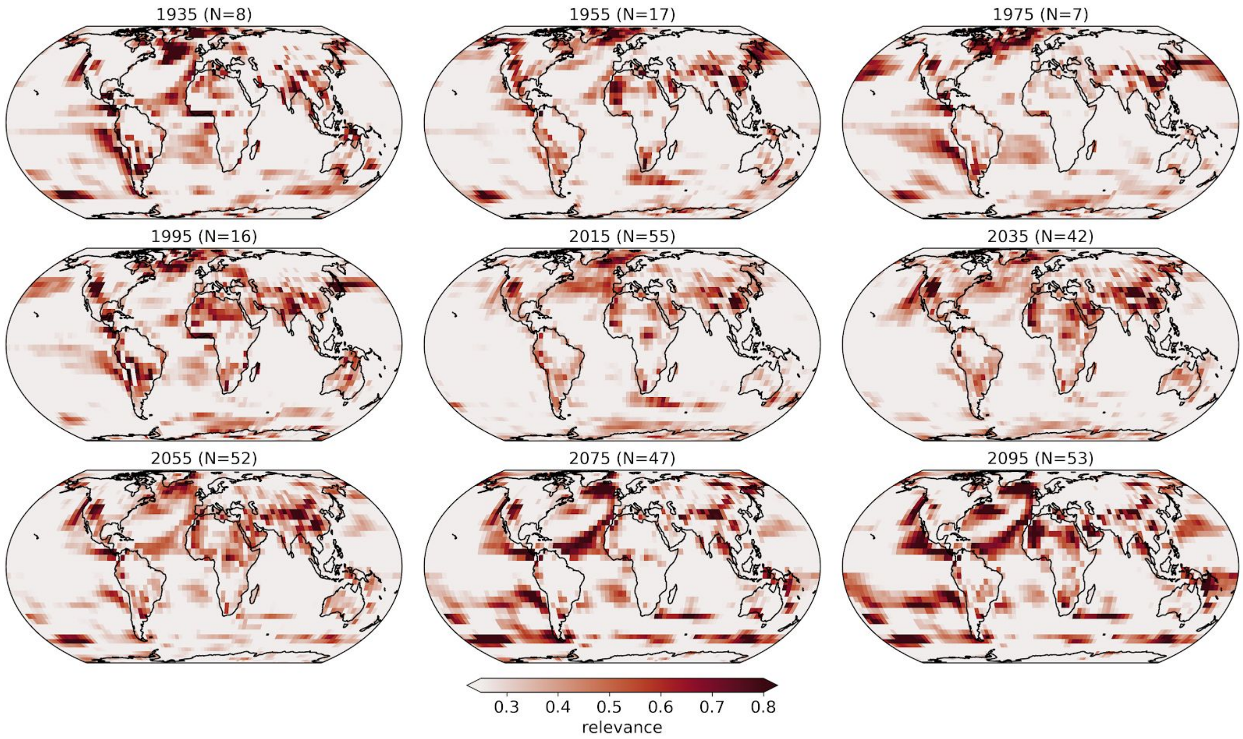


**Supp. Figure 4: Temperature, global mean removed.** Layerwise relevance propagation (LRP) heatmaps for temperature input maps where the global mean has been removed from every map prior to training composited for a range of years when the prediction was deemed accurate (see text for details). The years are shown above each panel along with the number of maps composited. Darker shading denotes regions that are more relevant for the ANN's accurate prediction.

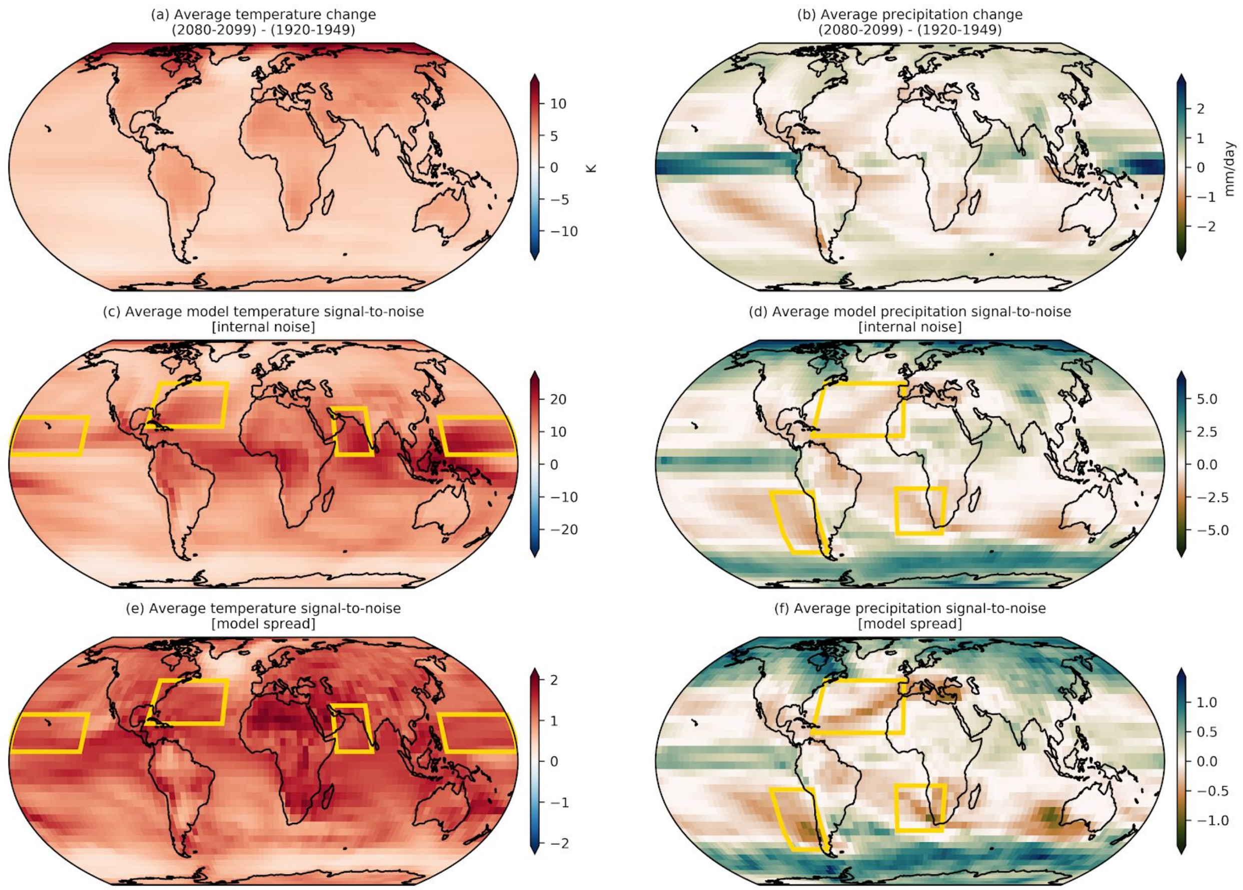


**Supp. Figure 5:** (a) Multi-model average change in temperature between 2070-2099 and 1920-1949. (c) The average across models of each model's signal-to-noise ratio, where the signal is defined by the change in temperature and the noise is defined by the internal noise of the model (see text for details). (e) The multi-model signal-to-noise ratio, where the signal is defined by the change in temperature and the noise is defined by total spread/range of change across models. (b,d,f) as in (a,c,e) except for precipitation. Yellow boxes denote example regions which show enhanced importance using LRP in Figures 6 and 13.

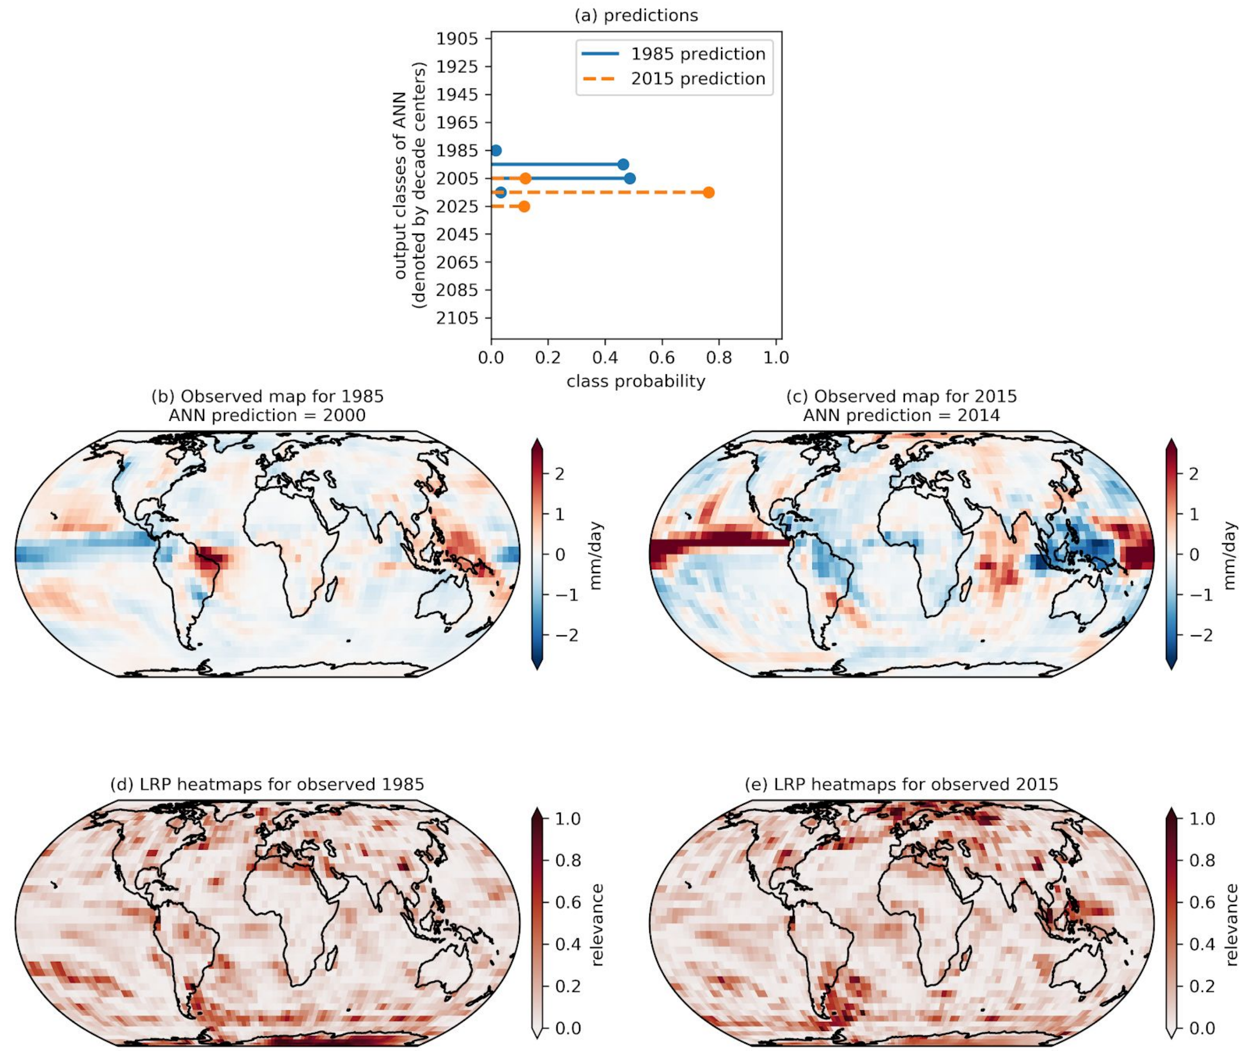


**Supp. Figure 6: Precipitation, global mean removed.** (a) Fuzzy classification output based on observed maps of 1985 and 2015. Tick marks on the y-axis list every 2nd class for space reasons. (b,c) Observed precipitation input maps plotted as anomalies from the baseline period of 1979-2099 where the global mean has been removed. (d,e) Layerwise relevance propagation heatmap for the ANN's year prediction.

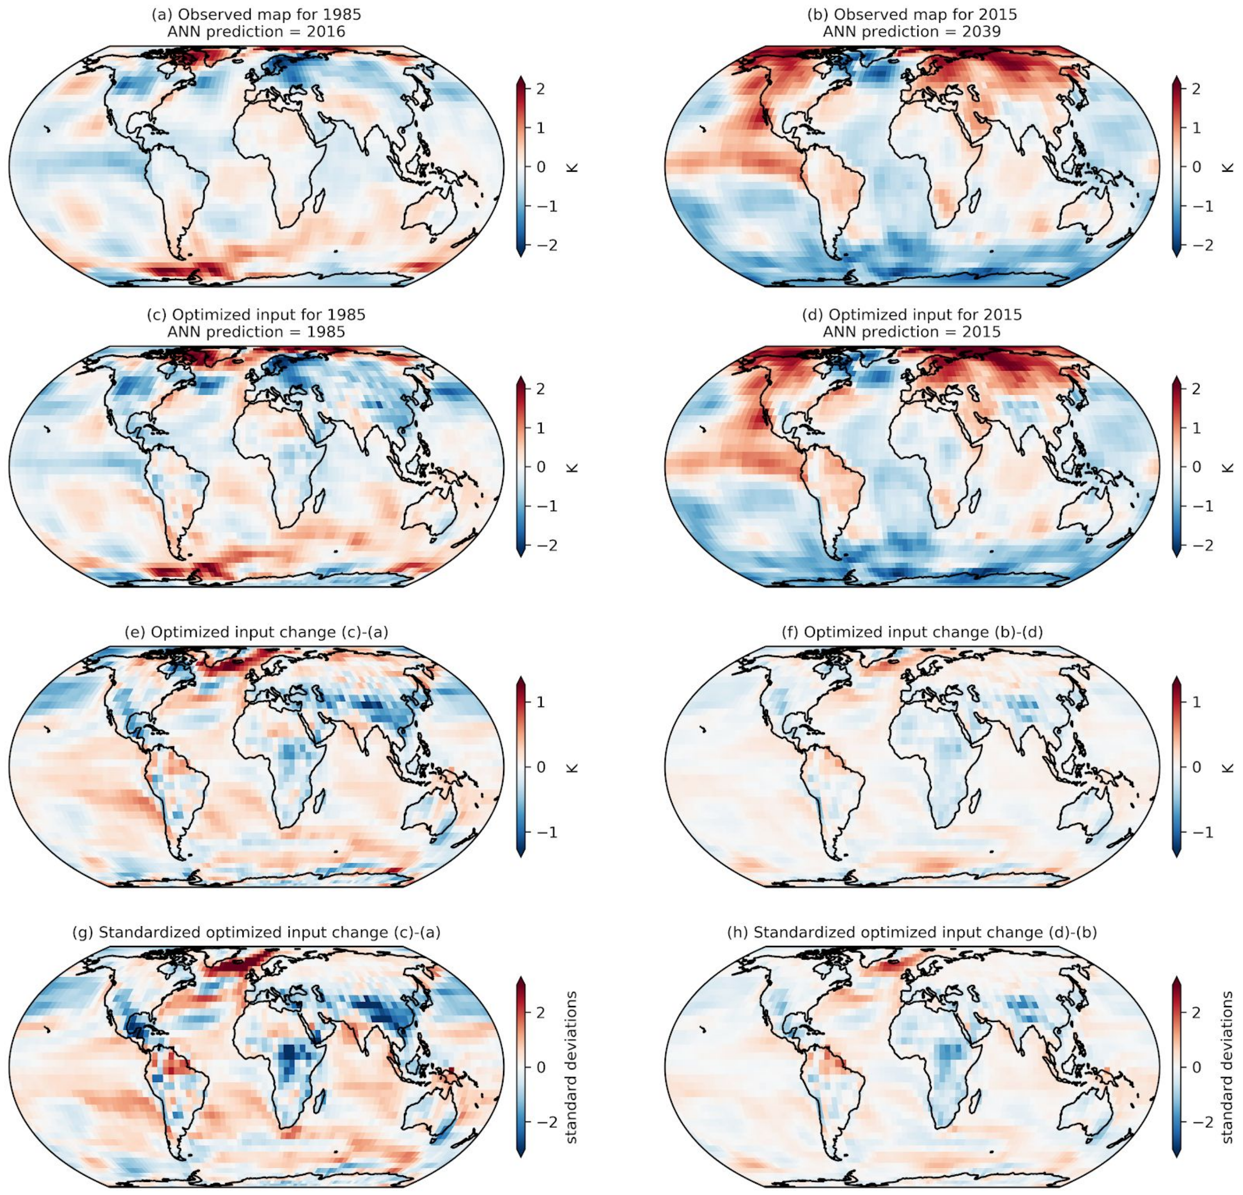


**Supp. Figure 7: Temperature, global mean removed.** (a,b) Observed BEST temperature anomaly maps plotted as anomalies from the baseline period of 1961-1990 where the global mean temperature has been removed. (c,d) Optimized input map determined using backward optimization. (e,f) Difference between observed map and optimal input. (g,h) Difference, but standardized by the local standard deviation, defined from detrended values over the baseline period. Left panel shows results for the observed input map from 1985, while right panel shows results for the observed input map from 2015. Both optimization procedures used 21 training iterations.

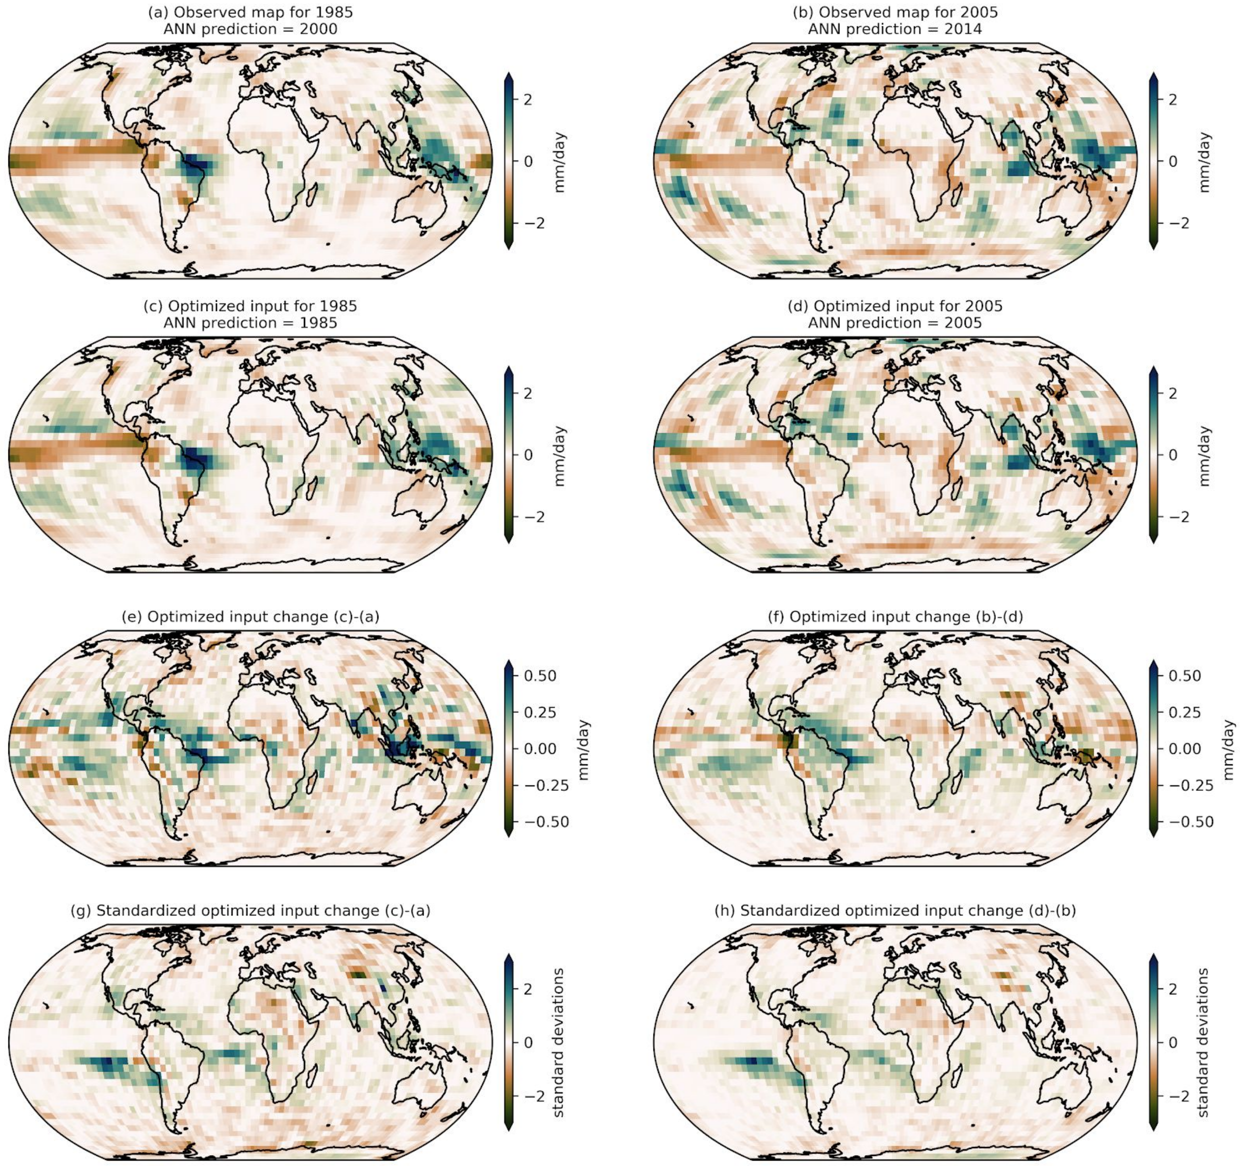


**Supp. Figure 8: Precipitation, global mean removed.** (a,b) Observed GPCP precipitation anomaly maps plotted as anomalies from the baseline period of 1979-1999 where the global mean precipitation has been removed. (c,d) Optimized input map determined using backward optimization. (e,f) Difference between observed map and optimal input. (g,h) Difference, but standardized by the local standard deviation, defined from detrended values over the baseline period. Left panel shows results for the observed input map from 1985 (42 optimization iterations), while right panel shows results for the observed input map from 2005 (21 optimization iterations).

## Tables S1-S2

**Supplemental Table 1:** 29 CMIP5 models analyzed with available temperature data. A single ensemble member for each model was analyzed. Specifics about each model, its institution can be found at https://cmip.llnl.gov/cmip5/docs/CMIP5_modeling_groups.pdf.

1. ACCESS1-0
2. ACCESS1-3
3. CCSM4
4. CESM1-BGC
5. CESM1-CAM5
6. CMCC-CMS
7. CNRM-CM5
8. CSIRO-Mk3-6-0
9. CanESM2
10. GFDL-CM3
11. GFDL-ESM2G
12. GFDL-ESM2M
13. GISS-E2-H-CC
14. GISS-E2-H
15. GISS-E2-R-CC
16. GISS-E2-R
17. HadGEM2-AO
18. HadGEM2-CC
19. HadGEM2-ES
20. inmcm4
21. IPSL-CM5A-LR
22. IPSL-CM5A-MR
23. MIROC-ESM-CHEM
24. MIROC-ESM
25. MIROC5
26. MPI-ESM-MR
27. MRI-CGCM3
28. NorESM1-M
29. NorESM1-ME

**Supplemental Table 2:** 22 CMIP5 models analyzed with available precipitation data. A single ensemble member for each model was analyzed. Specifics about each model and its institution can be found at https://cmip.llnl.gov/cmip5/docs/CMIP5_modeling_groups.pdf.

1. ACCESS1-0
2. ACCESS1-3
3. CMCC-CMS
4. CNRM-CM5
5. CSIRO-Mk3-6-0
6. CanESM2
7. GFDL-CM3
8. GFDL-ESM2G
9. GFDL-ESM2M
10. GISS-E2-H-CC
11. GISS-E2-H
12. GISS-E2-R-CC
13. GISS-E2-R
14. HadGEM2-CC
15. HadGEM2-ES
16. inmcm4
17. MIROC-ESM-CHEM
18. MIROC-ESM
19. MIROC5
20. MRI-CGCM3
21. NorESM1-M
22. NorESM1-ME
